# Supplementary material for: Strain Effects on Phase Transitions in Transition Metal Dichalcogenides
Source: arXiv:1811.05122 source file (2019-03-19)
Supplement: Supplementary file 1 [file SI.pdf]

Supplementary Information:  
Strain Effects on Phase Transitions in Transition Metal  
Dichalcogenides

Seoung-Hun Kang, Young-Kyun Kwon\*

*Department of Physics and Research Institute for Basic Sciences, Kyung Hee University, Seoul,  
02447, Korea*

*Korea Institute for Advanced Study (KIAS), Seoul 02455, Korea*

---

---

---

\*Corresponding author.

*Email address:* ykkwon@khu.ac.kr (Young-Kyun Kwon)

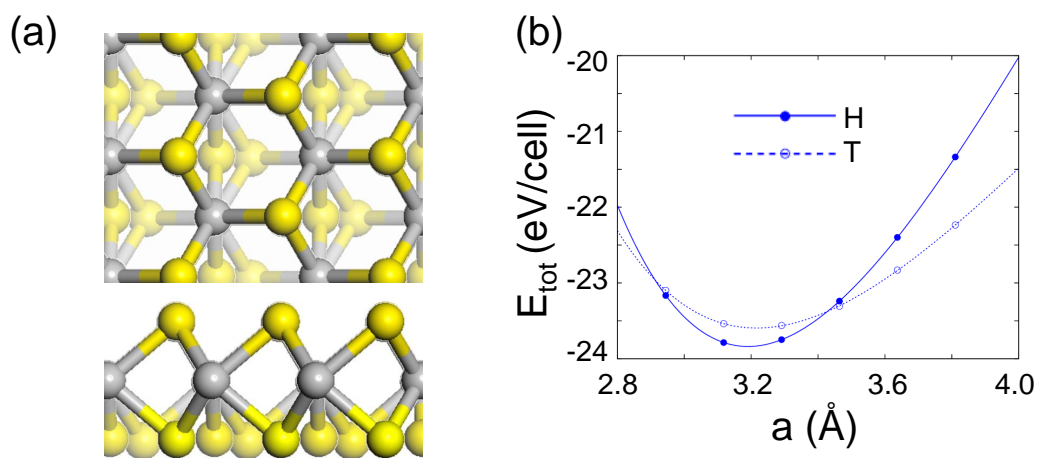

Figure S1: (a) Illustration of three steps of a considered phase transition pathway from the  $T$  phase to the  $H$  phase: top and side views. (b) Total Energy  $E_{\text{tot}}$  of the  $H$  (solid line) and  $T$  (dotted line) phases of  $\text{WS}_2$  as a function of lattice constants calculated with spin-orbit coupling.

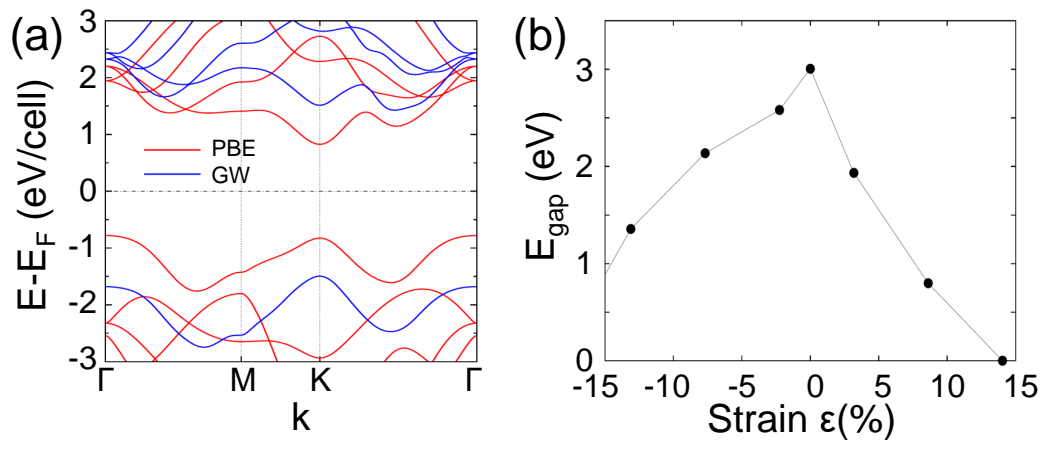

Figure S2: (a) Electronic band structures of the *H*-phase MoS<sub>2</sub> at equilibrium obtained from PBE functional (red) and *GW* correction (blue). (b) Electronic band gap as function of strain in the *H*-phase MoS<sub>2</sub> within *GW* correction.
